# Supplementary material for: Is being an only child harmful to psychological health?: Evidence from an instrumental variable analysis of China's One-Child Policy
Source: arXiv:2005.09130 source file (2020-06-11)
Supplement: Supplementary file 1 [file Supplementary2020.pdf]

# Supplementary material for “Is being the only child harmful for psychological health?: Evidence from an instrumental variable analysis of China’s One-Child Policy”

Shuxi Zeng
*Duke University, Durham, USA*
Fan Li
*Duke University, Durham, USA*
Peng Ding
*University of California, Berkeley, USA*

In the main paper, we only show the sensitivity analysis results for the effect on confidence measure and urban males subgroup under the violation of exclusion restriction assumption. We include the sensitivity analysis for other outcomes and subgroups in this document. Likewise, we vary the sensitivity parameter $r$, which is the ratio of direct effect from instrumental variable and the total effect in pyschological health, from $-0.5$ to $0.5$. Figures 1,2 and 3 show the relationships between the estimated causal effects of being the only child and the sensitivity parameter $r$ for the confidence, anxiety and desperate measures, respectively.

The x-axis is the value of sensitivity parameter $r$, which describes how much impact on the psychological health can be explained by the instrumental variable itself. Exclusion restriction assumption hold when $r = 0$ and a larger value indicates a stronger violation of the assumption. When $r$ is close to 1, a larger proportion of effect can be explained by the instrumental variable without passing through the treatment, the impact from being the only child on the pyschological measure shrinks to zero. This explains the pattern we observe in each graph. For those outcome measures and subgroups with significantly negative effects of being the only child when $r = 0$, the estimated effect remains significantly negative provided that $r$ is smaller than $5 - 10\%$. Hence, as long as the direct effect of instrumental variable does not take up more than $10\%$ of the total effect, the influence from being the only child remains negative even under the violation of exclusion restriction assumption.

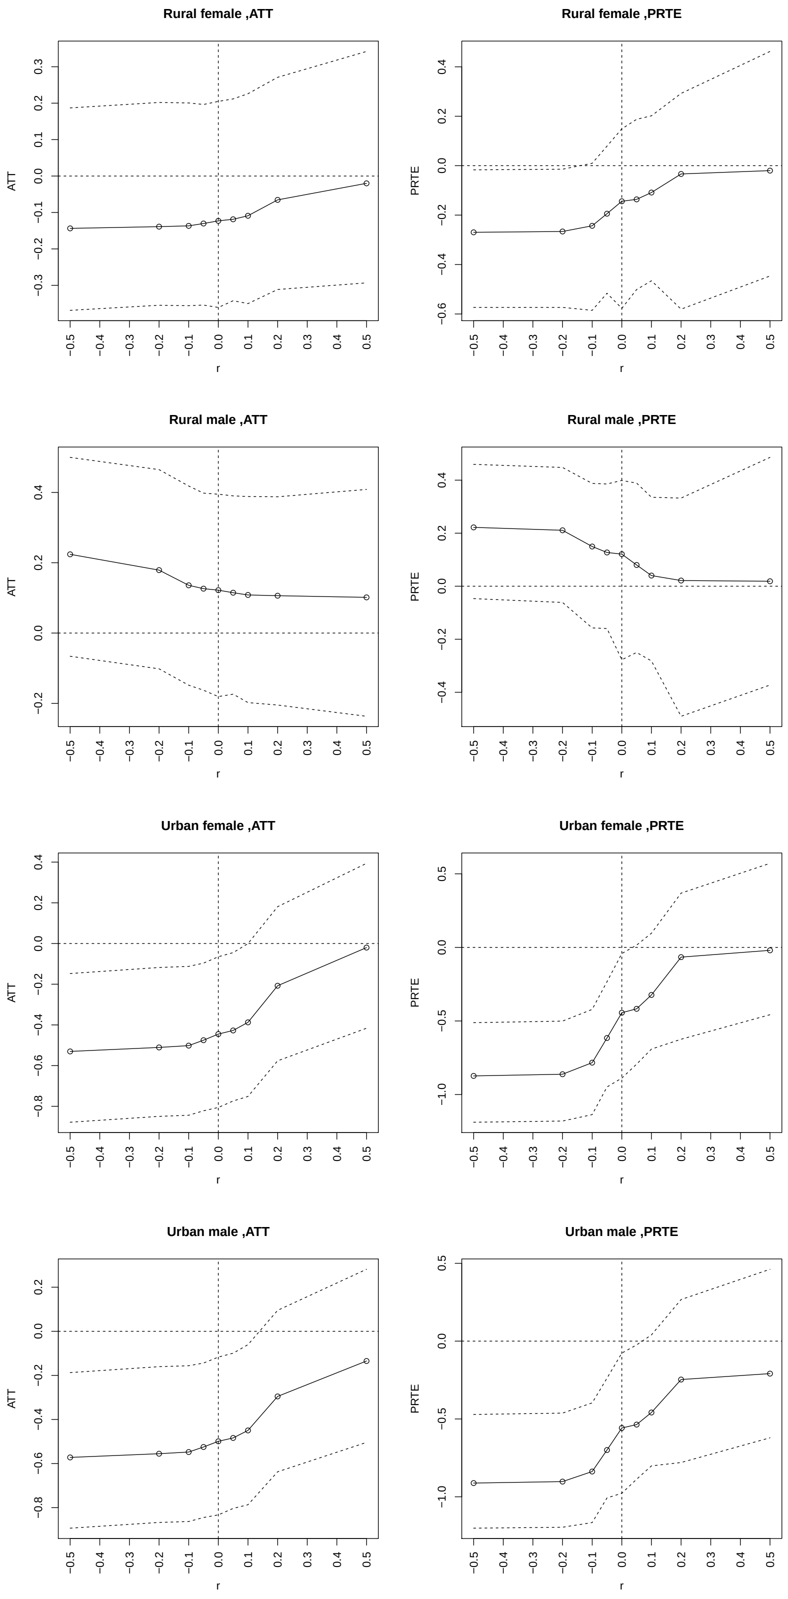


**Fig. 1.** Posterior means and 95% credible intervals of $\tau^{\mathrm{ATT}}$ and $\tau^{\mathrm{PRTE}}$ against the sensitivity parameter $r$, 4 subgroups (from top to bottom: rural female, rural male, urban female, urban male)

.

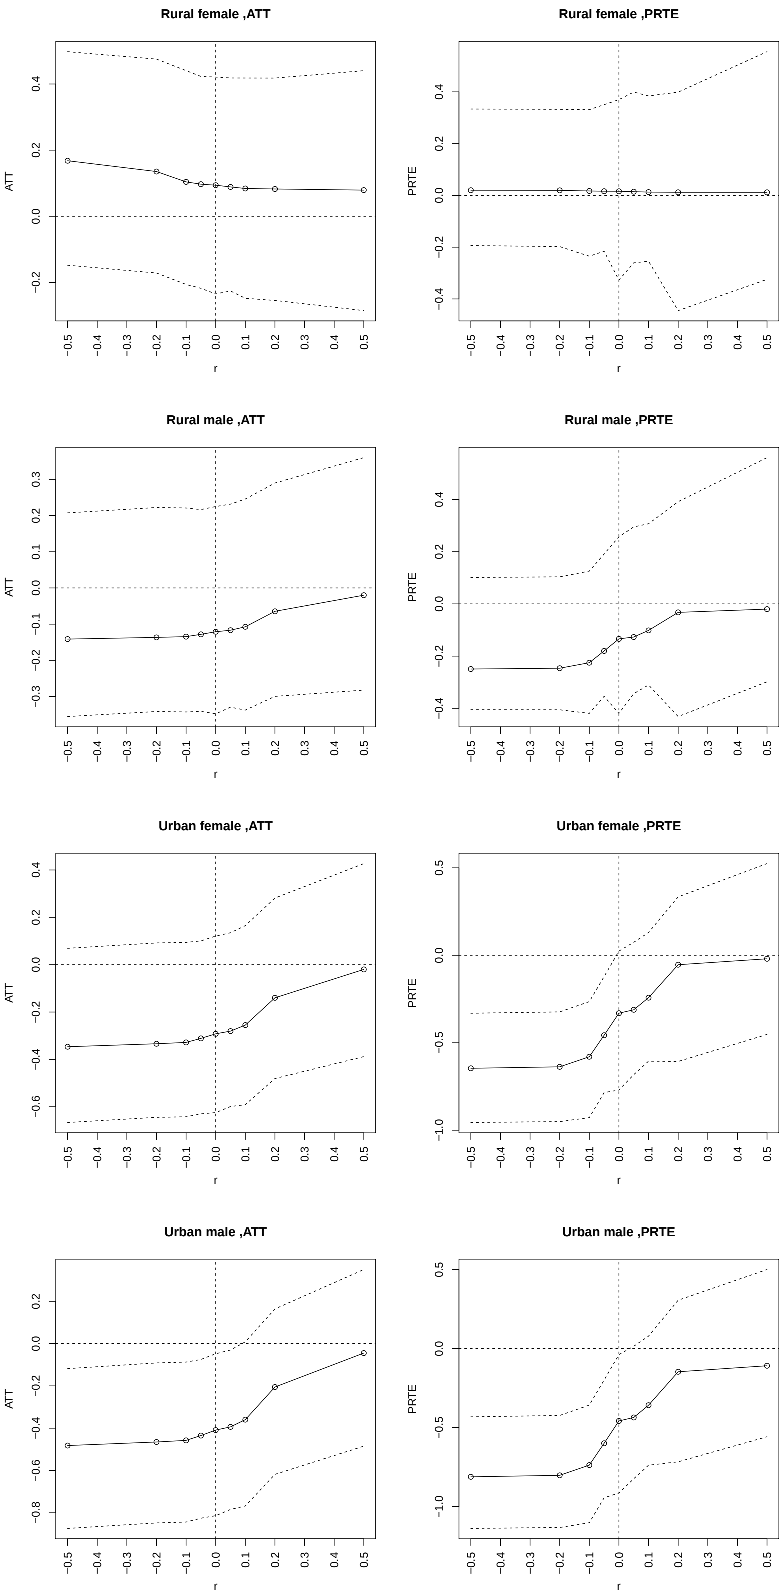


**Fig. 2.** Posterior means and 95% credible intervals of $\tau^{\text{ATT}}$ and $\tau^{\text{PRTE}}$ against the sensitivity parameter $r$, 4 subgroups (from top to bottom: rural female, rural male, urban female, urban male)

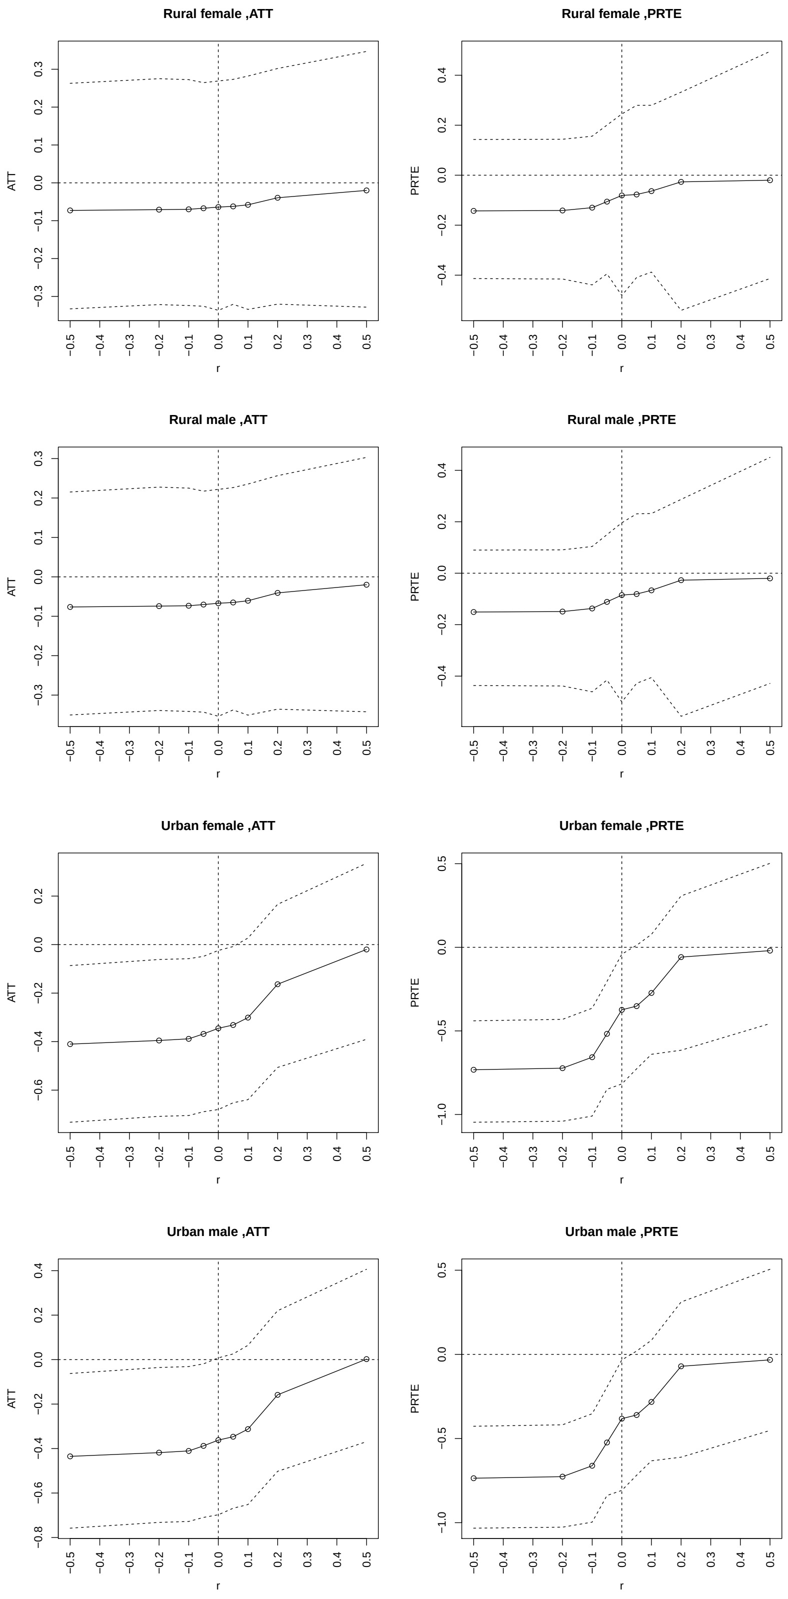


**Fig. 3.** Posterior means and 95% credible intervals of $\tau^{\text{ATT}}$ and $\tau^{\text{PRTE}}$ against the sensitivity parameter $r$, 4 subgroups (from top to bottom: rural female, rural male, urban female, urban male)

.
